# Supplementary material for: Improved Grid Optimization and Fitting in Least Squares Tensor Hypercontraction
Source: arXiv:1912.02120 source file (2019-12-04)
Supplement: Supplementary file 1 [file supporting_information.pdf]

# Improved Grid Optimization and Fitting in Least Squares Tensor Hypercontraction: Supplemental Information

Devin A. Matthews*

*Southern Methodist University, Dallas, TX 75275, USA*

## 1 Molecular Geometries

The utilized geometry for all-trans retinal is (in Å units):

| | | | |
|---|---|---|---|
| O | 8.7049 | −1.1237 | 0.6412 |
| C | −4.5389 | 0.8655 | 0.3849 |
| C | −5.9341 | 0.1864 | 0.3140 |
| C | −5.8892 | −1.2663 | 0.7527 |
| C | −3.4322 | −0.0455 | −0.1964 |
| C | −4.9519 | −2.0545 | −0.1496 |
| C | −3.6406 | −1.3604 | −0.4585 |
| C | −4.2148 | 1.1952 | 1.8602 |
| C | −4.6713 | 2.1943 | −0.3987 |
| C | −2.1452 | 0.5928 | −0.4196 |
| C | −2.6368 | −2.3078 | −1.0741 |
| C | −0.9729 | 0.0016 | −0.1375 |
| C | 0.3573 | 0.5792 | −0.3330 |
| C | 0.4314 | 1.9762 | −0.9060 |
| C | 1.5117 | −0.0553 | −0.0335 |
| C | 2.8738 | 0.4244 | −0.1876 |
| C | 3.9448 | −0.3151 | 0.1525 |
| C | 5.3470 | 0.0840 | 0.0342 |
| C | 5.6362 | 1.4589 | −0.5235 |
| C | 6.3923 | −0.6896 | 0.3876 |
| C | 7.8287 | −0.3403 | 0.2909 |
| H | −6.3192 | 0.2275 | −0.7146 |
| H | −6.6580 | 0.7312 | 0.9333 |
| H | −6.8938 | −1.7028 | 0.7086 |

*Electronic address: damatthews@smu.edu

| | | | |
|---|---|---|---|
| H | −5.5615 | −1.3434 | 1.7957 |
| H | −5.4596 | −2.2658 | −1.0997 |
| H | −4.7544 | −3.0224 | 0.3279 |
| H | −5.0191 | 1.7805 | 2.3205 |
| H | −4.0754 | 0.2892 | 2.4598 |
| H | −3.2953 | 1.7861 | 1.9462 |
| H | −5.5615 | 2.7493 | −0.0783 |
| H | −3.8175 | 2.8608 | −0.2355 |
| H | −4.7635 | 2.0145 | −1.4761 |
| H | −2.1640 | 1.5769 | −0.8729 |
| H | −2.1282 | −2.8893 | −0.2989 |
| H | −1.9016 | −1.8125 | −1.7132 |
| H | −3.1508 | −3.0176 | −1.7337 |
| H | −0.9559 | −0.9717 | 0.3477 |
| H | 1.4240 | 2.4097 | −1.0168 |
| H | −0.1241 | 2.6726 | −0.2661 |
| H | −0.0199 | 1.9942 | −1.9053 |
| H | 1.4334 | −1.0622 | 0.3788 |
| H | 3.0332 | 1.4134 | −0.5929 |
| H | 3.7867 | −1.3130 | 0.5601 |
| H | 5.1680 | 2.2224 | 0.1097 |
| H | 5.2145 | 1.5465 | −1.5323 |
| H | 6.6781 | 1.7544 | −0.6168 |
| H | 6.2046 | −1.6829 | 0.7907 |
| H | 8.1059 | 0.6427 | −0.1022 |

The geometry for benzene used $R_{CC} = 1.39\,\text{Å}$ and $R_{CH} = 1.09\,\text{Å}$.

# 2 Grid Generation and Laplace Quadrature

The parent grid for retinal was chosen as a Becke-type grid with a 29-point Treutler-Ahlrichs radial quadrature[1] for C and O (21 radial points for H) and a Lebedev angular quadrature.[2] The size of the angular quadrature was determined by the profile,[3]

$$L(x) = \lfloor L_{\max}(\mathrm{erf}(1.2x) - 0.5\mathrm{erf}(1.2x - 3) - 0.5) \rfloor$$

where $L$ is the highest angular momentum through which the angular quadrature is exact and $x = r/R$ is the reduced radial coordinate. The atomic radii $R$ are chosen as the standard Bragg-Slater radii and $L_{\max} = 17$ was used. This grid has 49527 total points (1011 points/atom, $n_{P'}/n_{DF} = 31.6$). A 9-point Braess-Hackbusch quadrature[4] was used for the Laplace transform of the energy denominators.

The parent grids for the benzene calculations are constructed similarly, with the only differences being the number of radial quadrature points ($n_{rad}$(C) and $n_{rad}$(H)) and the

| Name | $L_{\max}$ | $n_{rad}$(H) | $n_{rad}$(C) | $n_{P'}$ | $n_P^{(ai\|}$ | | | | |
|---|---|---|---|---|---|---|---|---|---|
| | | | | | X = D | X = T | X = Q | X = 5 | X = 6 |
| Grid1 | 7 | 11 | 19 | 2248 | 1244 | 1692 | 1806 | 1850 | 1924 |
| Grid2 | 8 | 13 | 21 | 2534 | 1296 | 1864 | 2034 | 2094 | 2162 |
| Grid3 | 9 | 15 | 23 | 3120 | 1335 | 2164 | 2486 | 2602 | 2693 |
| Grid4 | 10 | 17 | 25 | 3576 | 1348 | 2284 | 2746 | 2955 | 3088 |
| Grid5 | 11 | 19 | 27 | 4338 | 1373 | 2645 | 3292 | 3638 | 3826 |
| Grid6 | 12 | 21 | 29 | 4812 | 1373 | 2669 | 3440 | 3928 | 4176 |
| Grid7 | 13 | 23 | 31 | 5814 | 1375 | 2778 | 3752 | 4402 | 4885 |
| Grid8 | 14 | 25 | 33 | 6898 | 1378 | 2937 | 4068 | 4880 | 5560 |
| Grid9 | 15 | 27 | 35 | 7876 | 1380 | 2951 | 4174 | 5142 | 5923 |
| Grid10 | 16 | 29 | 37 | 8918 | 1377 | 2993 | 4295 | 5341 | 6254 |
| Grid11 | 17 | 31 | 39 | 9976 | 1377 | 3012 | 4361 | 5479 | 6498 |
| Grid12 | 18 | 33 | 41 | 11278 | 1376 | 3013 | 4384 | 5481 | 6581 |
| Grid13 | 19 | 35 | 43 | 12710 | 1380 | 3024 | 4550 | 5910 | 7067 |
| Grid14 | 20 | 37 | 45 | 14664 | 1378 | 3029 | 4585 | 5924 | 7139 |
| Grid15 | 21 | 39 | 47 | 16530 | 1378 | 3011 | 4630 | 6117 | 7360 |
| Grid16 | 22 | 41 | 49 | 18132 | 1377 | 2997 | 4635 | 6204 | 7433 |
| Grid17 | 23 | 43 | 51 | 19770 | 1376 | 2990 | 4631 | 6233 | 7558 |

Table 1: Parent grids used in LS-THC-DF-MP2 calculations on benzene. See text for details.

maximum angular momentum $L_{\max}$. These values for all 17 grids are summarized in table 1. This table also includes the total number of parent grid points, as well as the size of the pruned $(ai|$ grids for each cc-pVXZ basis set.

# 3 Details of the Cholesky-Based Algorithm

The procedure for using the Cholesky decomposition of $S$ is outlined in the following pseudocode. The function BUILD_E is assumed to be a MO-based algorithm using pre-determined density fitting factors, but in general it may be any suitable algorithm.

**function** PRUNE_GRID($\{\phi_\mu\}$,$\{x_{P'}\}$,$C^p_\mu$,$C^q_\mu$)
  $X_p^{P'} = \sum_\mu C^p_\mu \phi_\mu(x_{P'})$
  $X_q^{P'} = \sum_\mu C^q_\mu \phi_\mu(x_{P'})$
  $S'_{P'Q'} = \sum_{pq} X_p^{P'} X_q^{P'} X_p^{Q'} X_q^{Q'}$
  Solve $S' = \Pi(R')^T R' \Pi^{-1}$ with relative tolerance $\epsilon$ on diagonal elements of $R'$
    ▷ E.g. `dpstrf` from LAPACK (note this function requires a cutoff $\epsilon^2 \|S\|_{\max}$)
  $n_P \leftarrow \mathrm{nrow}(R')$, $R \leftarrow R'_{:,1:n_P}$
  Select $X_p^P = \sum_{P'} X_p^{P'} \Pi_{P'P}$
  Select $X_q^P = \sum_{P'} X_q^{P'} \Pi_{P'P}$
  **return** $X_p^P$, $X_q^P$, $R$
**end function**

**function** BUILD_E($X_p^P$, $X_q^P$, $X_r^Q$, $X_s^Q$, $B^J_{pq}$, $B^J_{rs}$)
  $C^J_P = \sum_{pq} B^J_{pq} X_p^P X_q^P$
  $D^J_Q = \sum_{rs} B^J_{rs} X_r^Q X_s^Q$
  $E_{PQ} = \sum_J C^J_P D^J_Q$
  **return** $E$
**end function**

**function** SOLVE_CHOL($E$,$R_1$,$R_2$)
  Solve $R_1^T Z = E$
  Solve $Y R_2 = Z$
  Solve $R_1 W = Y$
  Solve $V R_2^T = W$
  **return** $V$
**end function**

**function** LS_THC_CHOL($\{\phi_\mu\}$, $\{x_{P'}\}$, $C^p_\mu$, $C^q_\mu$, $C^r_\mu$, $C^s_\mu$, $B^J_{pq}$, $B^J_{rs}$)
  $X_p^P, X_q^P, R_1 \leftarrow$ PRUNE_GRID($\{\phi_\mu\}$, $\{x_{P'}\}$, $C^p_\mu$, $C^q_\mu$)
  $X_r^Q, X_s^Q, R_2 \leftarrow$ PRUNE_GRID($\{\phi_\mu\}$, $\{x_{P'}\}$, $C^r_\mu$, $C^s_\mu$)
  $E \leftarrow$ BUILD_E($X_p^P$, $X_q^P$, $X_r^Q$, $X_s^Q$, $B^J_{pq}$, $B^J_{rs}$)
  $V \leftarrow$ SOLVE_CHOL($E$,$R_1$,$R_2$)
  **return** $V$, $X_p^P$, $X_q^P$, $X_r^Q$, $X_s^Q$
**end function**

# 4 Detailed Results: Retinal

Tables 2 and 3 detail the results for retinal/cc-pVDZ(-RI) including canonical DF-MP2 correlation energy and LS-THC-DF-MP2 correlation energy and grid sizes as a function of $\epsilon$. The reference energy is not reported; the current rather primitive implementation of density fitting in CFOUR only allows one auxiliary basis set and also does not allow mixing a density fitted correlation energy with conventional SCF, so the RI fitting basis was used for the DF-SCF step as well. A future implementation will use proper J/K fitting basis sets or conventional SCF. Figure 1 shows the size of the pruned grids as a function of $\epsilon$. The dotted region of the curves (where $\epsilon \gtrsim 0.01$) are not considered reliable based on the achieved accuracy—this is furthered evidenced by the departure of the curves from linearity in this region. The solid parts of the curves were fit with a linear regression, discussed further in the main text.

| | |
|---|---|
| $E^{corr}_{DF-MP2}$ / $\mathrm{E_h}$ | -2.921655474 |
| $n_o$ | 57 |
| $n_v$ | 356 |
| $n_{DF}$ | 1568 |
| $n_{P'}$ | 49527 |

Table 2: General parameters and canonical DF-MP2 correlation energy for retinal/cc-pVDZ(-RI).

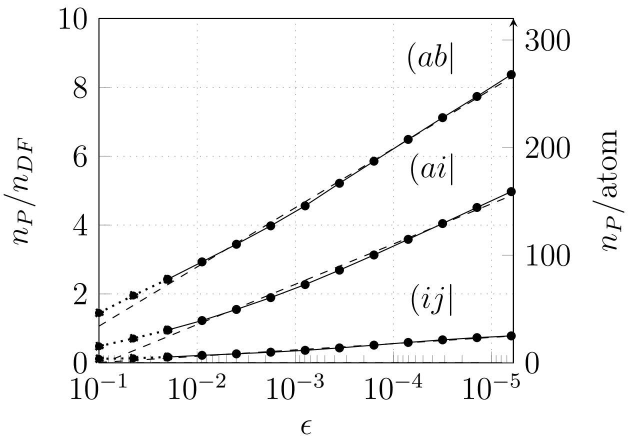


Figure 1: Number of points in the pruned grids as a function of $\epsilon$. The grid sizes are plotted relative to the size of the density fitting auxiliary basis ($n_{DF}$) and by average number of points per atom. Grids specialized to the $(ab|$, $(ai|$, and $(ij|$ charge distributions are generated, but note that the LS-THC-DF-MP2 results depend only on the $(ai|$ grid. Linear fits of the solid regions of the curves are plotted for reference (see text for details).

| Grid | $E^{corr}_{LS-THC-DF-MP2}$ / $\mathrm{E_h}$ | $\Delta E$ / $\mathrm{E_h}$ | $n_P^{(ab\|}$ | $n_P^{(ai\|}$ | $n_P^{(ij\|}$ |
|---|---|---|---|---|---|
| 1.00E-01 | -2.673013315 | 2.486E-01 | 2268 | 751 | 180 |
| 4.47E-02 | -2.874778209 | 4.688E-02 | 3064 | 1106 | 205 |
| 2.00E-02 | -2.918126551 | 3.529E-03 | 3801 | 1489 | 262 |
| 8.91E-03 | -2.921207696 | 4.478E-04 | 4596 | 1923 | 340 |
| 3.98E-03 | -2.921578518 | 7.696E-05 | 5397 | 2429 | 407 |
| 1.78E-03 | -2.921647637 | 7.837E-06 | 6237 | 2968 | 482 |
| 7.94E-04 | -2.921654487 | 9.862E-07 | 7148 | 3562 | 568 |
| 3.55E-04 | -2.921655011 | 4.625E-07 | 8175 | 4218 | 677 |
| 1.58E-04 | -2.921655765 | -2.915E-07 | 9180 | 4909 | 803 |
| 7.08E-05 | -2.921655556 | -8.232E-08 | 10172 | 5621 | 927 |
| 3.16E-05 | -2.921655479 | -5.569E-09 | 11163 | 6341 | 1045 |
| 1.41E-05 | -2.921655481 | -7.339E-09 | 12128 | 7073 | 1145 |
| 6.31E-06 | -2.921655476 | -1.996E-09 | 13124 | 7795 | 1225 |
| 2.82E-06 | -2.921655491 | -1.699E-08 | 14110 | 8519 | 1301 |
| 1.26E-06 | -2.921656143 | -6.693E-07 | 15111 | 9223 | 1374 |
| 5.62E-07 | -2.92168123 | -2.576E-05 | 16099 | 9936 | 1442 |
| 2.51E-07 | -2.921294603 | 3.609E-04 | 17084 | 10632 | 1505 |
| 1.12E-07 | -2.313218852 | 6.084E-01 | 18054 | 11308 | 1560 |
| 5.01E-08 | div. | — | 19023 | 11982 | 1601 |
| 2.24E-08 | div. | — | 19647 | 12514 | 1640 |
| 1.00E-08 | div. | — | 19712 | 12609 | 1674 |

Table 3: LS-THC-DF-MP2 correlation energy with absolute error and pruned grid sizes for retinal/cc-pVDZ(-RI) as a function of $\epsilon$.

# 5 Detailed Results: Benzene

Tables 4 and 5 detail the results for benzene/cc-pVXZ(-RI) including canonical DF-MP2 correlation energy and LS-THC-DF-MP2 correlation energy. The sizes of the pruned $(ai|$ grids for each grid/basis set combination are given above in Table 1. Figure 2(left) shows a more detailed analysis of grid size (expressed as $n_P^{(ai|}$/atom) versus achieved accuracy. The saturation of the pruned grid is clearly discernible for cc-pVTZ and cc-pVQZ (the cc-pVDZ grids are already saturated for the smallest parent grid), while saturation in the cc-pV5Z and cc-pV6Z basis sets is more subtle, appearing as a clustering of data points near 450 points/atom and 550 points/atom, respectively. The right panel shows the percentage of parent grid points pruned. The saturation points are clearly visible here as the pruning fraction rises rapidly from $\sim 15\%$ to $\sim 60\%$ with little change in accuracy.

| | cc-pVDZ | cc-pVTZ | cc-pVQZ | cc-pV5Z | cc-pV6Z |
|---|---|---|---|---|---|
| $E^{corr}_{DF-MP2}$ / $E_h$ | -0.782657720 | -0.949924419 | -1.009040486 | -1.031519840 | -1.041916251 |
| $n_o$ | 15 | 15 | 15 | 15 | 15 |
| $n_v$ | 93 | 243 | 489 | 855 | 1365 |
| $n_{DF}$ | 420 | 666 | 1122 | 1704 | 2538 |

Table 4: General parameters and canonical DF-MP2 correlation energy for benzene/cc-pVXZ(-RI).

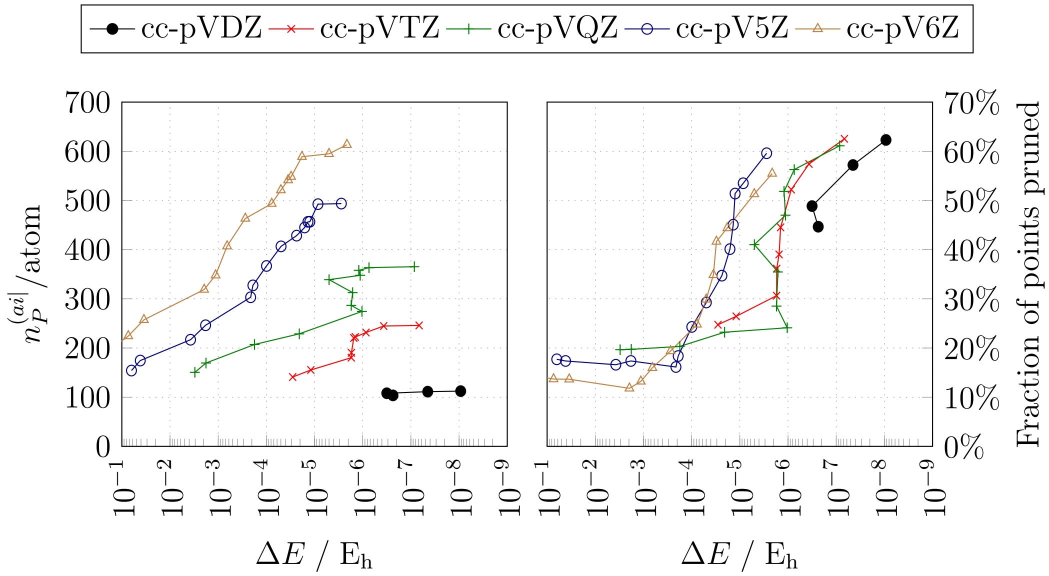


Figure 2: Accuracy of the LS-THC-DF-MP2 approximation compared to canonical DF-MP2 for benzene as a function the parent grid size and orbital basis set. The number of pruned grid points (for the $(ai|$ distribution—left) and the percentage of points pruned from the parent grid (right) are plotted versus the accuracy achieved. The grids used are described in the text, and $\epsilon = 10^{-5}$ is used throughout.

| Grid | $E^{corr}_{LS-THC-DF-MP2}$ / $E_h$ | | | | |
|---|---|---|---|---|---|
| | X = D | X = T | X = Q | X = 5 | X = 6 |
| Grid1 | -0.782657956 | -0.949895998 | -1.005990817 | -0.968465550 | -0.662370985 |
| Grid2 | -0.782658037 | -0.949912495 | -1.007250555 | -0.990128164 | -0.751530342 |
| Grid3 | -0.782657765 | -0.949922693 | -1.008864300 | -1.027771843 | -0.968448669 |
| Grid4 | -0.782657729 | -0.949926135 | -1.009019752 | -1.029693780 | -1.007169537 |
| Grid5 | -0.782657727 | -0.949922888 | -1.009039447 | -1.031307950 | -1.039960782 |
| Grid6 | -0.782657717 | -0.949922995 | -1.009038755 | -1.031329666 | -1.040783988 |
| Grid7 | -0.782657716 | -0.949923563 | -1.009038866 | -1.031420538 | -1.041262846 |
| Grid8 | -0.782657733 | -0.949924052 | -1.009035495 | -1.031470303 | -1.041642559 |
| Grid9 | -0.782657729 | -0.949924352 | -1.009039358 | -1.031496261 | -1.041838929 |
| Grid10 | -0.782657717 | -0.949924425 | -1.009039277 | -1.031503803 | -1.041866321 |
| Grid11 | -0.782657713 | -0.949924359 | -1.009041227 | -1.031506139 | -1.041880867 |
| Grid12 | -0.782657718 | -0.949924392 | -1.009040570 | -1.031507306 | -1.041885645 |
| Grid13 | -0.782657713 | -0.949924353 | -1.009041016 | -1.031511340 | -1.041898011 |
| Grid14 | -0.782657727 | -0.949924364 | -1.009039943 | -1.031517063 | -1.041911242 |
| Grid15 | -0.782657726 | -0.949924300 | -1.009040125 | -1.031517563 | -1.041914121 |
| Grid16 | -0.782657711 | -0.949924365 | -1.009040350 | -1.031517787 | -1.041911745 |
| Grid17 | -0.782657715 | -0.949924319 | -1.009040025 | -1.031517800 | -1.041914038 |

| Grid | $\Delta E$ / $E_h$ | | | | |
|---|---|---|---|---|---|
| | X = D | X = T | X = Q | X = 5 | X = 6 |
| Grid1 | -2.359E-07 | 2.842E-05 | 3.050E-03 | 6.305E-02 | 3.795E-01 |
| Grid2 | -3.166E-07 | 1.192E-05 | 1.790E-03 | 4.139E-02 | 2.904E-01 |
| Grid3 | -4.478E-08 | 1.727E-06 | 1.762E-04 | 3.748E-03 | 7.347E-02 |
| Grid4 | -9.260E-09 | -1.716E-06 | 2.073E-05 | 1.826E-03 | 3.475E-02 |
| Grid5 | -7.287E-09 | 1.531E-06 | 1.038E-06 | 2.119E-04 | 1.955E-03 |
| Grid6 | 2.536E-09 | 1.425E-06 | 1.730E-06 | 1.902E-04 | 1.132E-03 |
| Grid7 | 4.451E-09 | 8.558E-07 | 1.620E-06 | 9.930E-05 | 6.534E-04 |
| Grid8 | -1.287E-08 | 3.670E-07 | 4.991E-06 | 4.954E-05 | 2.737E-04 |
| Grid9 | -8.825E-09 | 6.747E-08 | 1.127E-06 | 2.358E-05 | 7.732E-05 |
| Grid10 | 2.862E-09 | -6.241E-09 | 1.209E-06 | 1.604E-05 | 4.993E-05 |
| Grid11 | 6.685E-09 | 6.069E-08 | -7.415E-07 | 1.370E-05 | 3.538E-05 |
| Grid12 | 1.976E-09 | 2.720E-08 | -8.473E-08 | 1.253E-05 | 3.061E-05 |
| Grid13 | 6.680E-09 | 6.667E-08 | -5.301E-07 | 8.500E-06 | 1.824E-05 |
| Grid14 | -7.216E-09 | 5.557E-08 | 5.424E-07 | 2.776E-06 | 5.009E-06 |
| Grid15 | -6.491E-09 | 1.193E-07 | 3.607E-07 | 2.277E-06 | 2.130E-06 |
| Grid16 | 9.341E-09 | 5.417E-08 | 1.352E-07 | 2.053E-06 | 4.506E-06 |
| Grid17 | 5.089E-09 | 9.985E-08 | 4.608E-07 | 2.040E-06 | 2.213E-06 |

Table 5: LS-THC-DF-MP2 correlation energy with absolute error for benzene with all cc-pVXZ basis sets, X = D, T, Q, 5, 6.

# References


[1] Treutler, O.; Ahlrichs, R. Efficient Molecular Numerical Integration Schemes. *J. Chem. Phys.* **1995**, *102*, 346–354.

[2] Lebedev, V. I. Quadratures on a Sphere. *USSR Computational Mathematics and Mathematical Physics* **1976**, *16*, 10–24.

[3] Parrish, R. M.; Hohenstein, E. G.; Martínez, T. J.; Sherrill, C. D. Discrete Variable Representation in Electronic Structure Theory: Quadrature Grids for Least-Squares Tensor Hypercontraction. *J. Chem. Phys.* **2013**, *138*, 194107.

[4] Braess, D.; Hackbusch, W. Approximation of 1/x by Exponential Sums in $[1, \infty)$. *IMA J Numer Anal* **2005**, *25*, 685–697.
